# Supplementary material for: TRUST: An LLM-Based Dialogue System for Trauma Understanding and Structured Assessments
Source: arXiv:2504.21851 source file (2025-04-30)
Supplement: Supplementary file 1 [file appendix.tex]

\section{Example Appendix}
\label{sec:appendix}

This is an appendix. \citet{louie-etal-2024-roleplay}
